# Supplementary material for: Pseudo-RIS: Distinctive Pseudo-supervision Generation for Referring Image Segmentation
Source: arXiv:2407.07412 source file (2024-07-17)
Supplement: Supplementary file 1 [file distinctiveness_datasets.tex]

\begin{table}[h]
    \centering
    \footnotesize
    \caption{Caption}
    \begin{tabular}{c|ccc}
    \hline
         & RefCOCO & RefCOCO+ & RefCOCOg \\ \hline
    Distinctiveness     & 1.018 & 1.046 & 1.124 \\
    \hline
    \end{tabular}
    \label{sup_tab:distinctiveness_datasets}
\end{table}
